# Supplementary material for: The Empty Signifier Problem: Towards Clearer Paradigms for Operationalising "Alignment" in Large Language Models
Source: arXiv:2310.02457 source file (2023-11-15)
Supplement: Supplementary file 1 [file appendix.tex]

\appendix
\section{Populating the Framework with Existing Literature}
\label{sec:lit_table}
\input{tables/2by2_solar}
